# Supplementary material for: Human Brains Can't Detect Fake News: A Neuro-Cognitive Study of Textual Disinformation Susceptibility
Source: arXiv:2207.08376 source file (2022-07-18)
Supplement: Supplementary file 1 [file Appendix.tex]

\newpage
\begin{appendices}
\section {Participant Demographics}
\label{Participant Demographics}
\begin{table}[htbp]
	\scriptsize
	\centering
	\caption{Summary of Participant Demographics}	
	\begin{tabular}{|l|l|r|}
		\hline
		\textbf{Demographics (N=19)}       &                                                                                                        & \textbf{\%}                                                       \\ \hline \hline
		 
		\textbf{Gender}                    & \begin{tabular}[c]{@{}l@{}}Male\\ Female\end{tabular}                                                  & \begin{tabular}[c]{@{}r@{}}57.9\\ 42.1\end{tabular}               \\ \hline
		 
		\textbf{Age}                       & \begin{tabular}[c]{@{}l@{}}18-24\\ 25-30\\ 31-40\\ \textgreater{}40\end{tabular}                       & \begin{tabular}[c]{@{}r@{}}26.3\\ 31.6\\ 21.1\\ 21.0\end{tabular} \\ \hline
		
		\textbf{Education}                 & \begin{tabular}[c]{@{}l@{}}Bachelor's degree\\ Master's degree\\ Doctoral degree\\ Others\end{tabular} & \begin{tabular}[c]{@{}r@{}}52.6\\ 26.3\\ 5.3\\ 15.8\end{tabular}  \\ \hline
		
		\textbf{Employement status}        & \begin{tabular}[c]{@{}l@{}}Employed\\ Non-Employed\end{tabular}                                        & \begin{tabular}[c]{@{}r@{}}31.6\\ 68.4\end{tabular}               \\ \hline
		
		\textbf{Frequency of Reading news} & \begin{tabular}[c]{@{}l@{}}Daily\\ Several times a week\\ Once a week\\ Others\end{tabular}            & \begin{tabular}[c]{@{}r@{}}21.1\\ 47.4\\ 21.1\\ 10.4\end{tabular} \\ \hline
		\textbf{Credibility of the News}   & \begin{tabular}[c]{@{}l@{}}Care\\ Do not care\end{tabular}                                             & \begin{tabular}[c]{@{}r@{}}73.7\\ 26.3\end{tabular}               \\ \hline
	\end{tabular}
	%\arrayrulecolor{black}	
	
	\label{particpantdemographics}
	%\vspace{-2mm}  
\end{table}

\end{appendices}
